# Supplementary material for: Active Information Gathering for Long-Horizon Navigation Under Uncertainty by Learning the Value of Information
Source: arXiv:2403.03269 source file (2024-03-05)
Supplement: Supplementary file 1 [file 9_appendix.tex]

\appendix
\section{Approach}
The value of information for an action depends on the planner's ability to use that information.
For example, a planner with a known map does not need to take an action that reveals a map telling the robot where the goal is, as it belief space remains the same. 
On the contrary, a planner without a complete map would find access to the map valuable to locate the goal quickly as it updates its belief space.
Given access to value of information for the actions with respect to a planner, we could learn them but value of information is computationally intractable.
So, we define the value of information for a planner as the difference between the expected planning cost without information and with information, we define it more formally later in Sec.~\ref{sec:eq-theory-value-of-info}.
